# Supplementary material for: On the efficacy of old features for the detection of new bots
Source: arXiv:2506.19635 source file (2025-06-24)
Supplement: Supplementary file 1 [file Appendix.tex]

\appendix

\begin{table*}[t!]
	\scriptsize
	\centering
	\begin{tabular}{lcccccc}
		\toprule
		& \multicolumn{5}{c}{\textbf{botwiki-celebrity}} \\
		\cmidrule{2-7}
		Name & Bal.Accuracy & Precision & Recall & MCC & PR-AUC & ROC-AUC \\
		\midrule
		ZeroR & 0,5 & 0 & 0 & 0 & 0,107 & 0,499 \\
\midrule 
\multicolumn{7}{l}{\texttt{CAP\_UNI}} \\
MultilayerPerceptron & 0,841 & 0,707 & 0,718 & 0,678 & 0,701 & 0,936 \\
JRip & 0,832 & 0,736 & 0,694 & 0,682 & 0,558 & 0,822 \\
NaiveBayes & 0,687 & 0,785 & 0,386 & 0,517 & 0,694 & 0,916 \\
RandomForest & 0,821 & 0,723 & 0,673 & 0,663 & 0,699 & 0,944 \\
IBk & 0,824 & 0,725 & 0,679 & 0,667 & 0,692 & 0,941 \\
\midrule 
\multicolumn{7}{l}{\texttt{ClassA}} \\
MultilayerPerceptron & 0,947 & 0,908 & 0,904 & 0,895 & 0,964 & 0,991 \\
JRip & 0,987 & 0,979 & 0,976 & 0,975 & 0,951 & 0,982 \\
NaiveBayes & 0,976 & 0,79 & 0,984 & 0,866 & 0,973 & 0,993 \\
RandomForest & 0,986 & 0,99 & 0,973 & 0,979 & 0,998 & 1 \\
IBk & 0,948 & 0,903 & 0,907 & 0,893 & 0,828 & 0,948 \\
\midrule 
\multicolumn{7}{l}{\texttt{ClassB}} \\
MultilayerPerceptron & 0,882 & 0,766 & 0,794 & 0,753 & 0,7 & 0,896 \\
JRip & 0,883 & 0,817 & 0,786 & 0,778 & 0,696 & 0,89 \\
NaiveBayes & 0,89 & 0,433 & 0,925 & 0,574 & 0,587 & 0,928 \\
RandomForest & 0,886 & 0,809 & 0,794 & 0,778 & 0,771 & 0,963 \\
IBk & 0,887 & 0,792 & 0,8 & 0,771 & 0,735 & 0,956 \\
\midrule 
\multicolumn{7}{l}{\texttt{\texttt{\% tweets by unofficial clients}}} \\
MultilayerPerceptron & 0,715 & 0,505 & 0,487 & 0,437 & 0,496 & 0,934 \\
JRip & 0,582 & 0,46 & 0,191 & 0,246 & 0,192 & 0,647 \\
NaiveBayes & 0,919 & 0,442 & 0,987 & 0,607 & 0,482 & 0,933 \\
RandomForest & 0,667 & 0,48 & 0,384 & 0,369 & 0,477 & 0,927 \\
IBk & 0,625 & 0,47 & 0,289 & 0,312 & 0,476 & 0,926 \\

	\bottomrule
	\end{tabular}
	\caption{\small botwiki-celebrity: 10-folds cross validation  (imbalanced, \#post > 10).}
	\label{tab:botwiki-celebrity10}
\end{table*}

\begin{table*}[t!]
	\scriptsize
	\centering
	\begin{tabular}{lcccccc}
		\toprule
		& \multicolumn{5}{c}{\textbf{botwiki-verified}} \\
		\cmidrule{2-7}
		Name & Bal.Accuracy & Precision & Recall & MCC & PR-AUC & ROC-AUC \\
		\midrule
		ZeroR & 0,5 & 0 & 0 & 0 & 0,251 & 0,499 \\
\midrule 
\multicolumn{7}{l}{\texttt{CAP\_UNI}} \\
MultilayerPerceptron & 0,841 & 0,876 & 0,715 & 0,732 & 0,857 & 0,913 \\
JRip & 0,839 & 0,884 & 0,709 & 0,733 & 0,76 & 0,836 \\
NaiveBayes & 0,713 & 0,97 & 0,431 & 0,587 & 0,841 & 0,888 \\
RandomForest & 0,845 & 0,875 & 0,724 & 0,736 & 0,866 & 0,919 \\
IBk & 0,845 & 0,875 & 0,724 & 0,736 & 0,862 & 0,919 \\
\midrule 
\multicolumn{7}{l}{\texttt{ClassA}} \\
MultilayerPerceptron & 0,946 & 0,92 & 0,919 & 0,893 & 0,945 & 0,984 \\
JRip & 0,981 & 0,973 & 0,97 & 0,962 & 0,976 & 0,985 \\
NaiveBayes & 0,958 & 0,899 & 0,952 & 0,899 & 0,964 & 0,982 \\
RandomForest & 0,981 & 0,988 & 0,966 & 0,969 & 0,997 & 0,999 \\
IBk & 0,952 & 0,913 & 0,933 & 0,896 & 0,868 & 0,954 \\
\midrule 
\multicolumn{7}{l}{\texttt{ClassB}} \\
MultilayerPerceptron & 0,934 & 0,931 & 0,89 & 0,881 & 0,932 & 0,961 \\
JRip & 0,934 & 0,932 & 0,89 & 0,882 & 0,894 & 0,935 \\
NaiveBayes & 0,913 & 0,73 & 0,942 & 0,764 & 0,79 & 0,942 \\
RandomForest & 0,938 & 0,915 & 0,904 & 0,879 & 0,94 & 0,979 \\
IBk & 0,939 & 0,895 & 0,913 & 0,871 & 0,896 & 0,966 \\
\midrule 
\multicolumn{7}{l}{\texttt{\texttt{\% tweets by unofficial clients}}} \\
MultilayerPerceptron & 0,907 & 0,677 & 0,969 & 0,736 & 0,671 & 0,912 \\
JRip & 0,907 & 0,677 & 0,969 & 0,736 & 0,643 & 0,895 \\
NaiveBayes & 0,889 & 0,612 & 0,987 & 0,686 & 0,656 & 0,91 \\
RandomForest & 0,907 & 0,677 & 0,969 & 0,736 & 0,652 & 0,907 \\
IBk & 0,907 & 0,677 & 0,969 & 0,736 & 0,648 & 0,905 \\

	\bottomrule
	\end{tabular}
	\caption{\small botwiki-verified: 10-folds cross validation  (imbalanced, \#post > 10).}
	\label{tab:botwiki-verified10}
\end{table*}

\begin{table*}[t!]
	\scriptsize
	\centering
	\begin{tabular}{lcccccc}
		\toprule
		& \multicolumn{5}{c}{\textbf{vendor-verified}} \\
		\cmidrule{2-7}
		Name & Bal.Accuracy & Precision & Recall & MCC & PR-AUC & ROC-AUC \\
		\midrule
		ZeroR & 0,5 & 0 & 0 & 0 & 0,232 & 0,499 \\
\midrule 
\multicolumn{7}{l}{\texttt{CAP\_UNI}} \\
MultilayerPerceptron & 0,908 & 0,947 & 0,83 & 0,856 & 0,931 & 0,952 \\
JRip & 0,903 & 0,955 & 0,817 & 0,852 & 0,871 & 0,896 \\
NaiveBayes & 0,876 & 0,983 & 0,755 & 0,828 & 0,919 & 0,942 \\
RandomForest & 0,898 & 0,946 & 0,81 & 0,842 & 0,928 & 0,953 \\
IBk & 0,9 & 0,944 & 0,815 & 0,844 & 0,928 & 0,954 \\
\midrule 
\multicolumn{7}{l}{\texttt{ClassA}} \\
MultilayerPerceptron & 0,885 & 0,897 & 0,798 & 0,803 & 0,912 & 0,954 \\
JRip & 0,925 & 0,931 & 0,868 & 0,87 & 0,901 & 0,933 \\
NaiveBayes & 0,715 & 0,946 & 0,437 & 0,586 & 0,877 & 0,953 \\
RandomForest & 0,937 & 0,947 & 0,888 & 0,893 & 0,968 & 0,983 \\
IBk & 0,867 & 0,83 & 0,783 & 0,75 & 0,709 & 0,866 \\
\midrule 
\multicolumn{7}{l}{\texttt{ClassB}} \\
MultilayerPerceptron & 0,76 & 0,861 & 0,547 & 0,619 & 0,769 & 0,847 \\
JRip & 0,745 & 0,797 & 0,531 & 0,572 & 0,643 & 0,752 \\
NaiveBayes & 0,774 & 0,719 & 0,621 & 0,577 & 0,634 & 0,803 \\
RandomForest & 0,757 & 0,714 & 0,584 & 0,552 & 0,715 & 0,824 \\
IBk & 0,75 & 0,627 & 0,611 & 0,505 & 0,651 & 0,8 \\
\midrule 
\multicolumn{7}{l}{\texttt{\texttt{\% tweets by unofficial clients}}} \\
MultilayerPerceptron & 0,5 & 0 & 0 & 0 & 0,359 & 0,69 \\
JRip & 0,5 & 0 & 0 & 0 & 0,232 & 0,499 \\
NaiveBayes & 0,5 & 0 & 0 & 0 & 0,354 & 0,677 \\
RandomForest & 0,5 & 0 & 0 & 0 & 0,353 & 0,701 \\
IBk & 0,5 & 0 & 0 & 0 & 0,352 & 0,7 \\

	\bottomrule
	\end{tabular}
	\caption{\small vendor-verified: 10-folds cross validation  (imbalanced, \#post > 10).}
	\label{tab:vendor-verified10}
\end{table*}

\begin{table*}[t!]
	\scriptsize
	\centering
	\begin{tabular}{lcccccc}
		\toprule
		& \multicolumn{5}{c}{\textbf{stock}} \\
		\cmidrule{2-7}
		Name & Bal.Accuracy & Precision & Recall & MCC & PR-AUC & ROC-AUC \\
		\midrule
		ZeroR & 0,5 & 0,551 & 1 & 0 & 0,55 & 0,5 \\
\midrule 
\multicolumn{7}{l}{\texttt{CAP\_UNI}} \\
MultilayerPerceptron & 0,724 & 0,71 & 0,895 & 0,483 & 0,703 & 0,736 \\
JRip & 0,725 & 0,717 & 0,871 & 0,474 & 0,707 & 0,732 \\
NaiveBayes & 0,709 & 0,72 & 0,798 & 0,426 & 0,662 & 0,714 \\
RandomForest & 0,726 & 0,715 & 0,884 & 0,482 & 0,748 & 0,775 \\
IBk & 0,725 & 0,714 & 0,883 & 0,48 & 0,748 & 0,775 \\
\midrule 
\multicolumn{7}{l}{\texttt{ClassA}} \\
MultilayerPerceptron & 0,698 & 0,733 & 0,712 & 0,394 & 0,776 & 0,756 \\
JRip & 0,808 & 0,825 & 0,832 & 0,615 & 0,807 & 0,83 \\
NaiveBayes & 0,535 & 0,569 & 0,987 & 0,167 & 0,738 & 0,725 \\
RandomForest & 0,822 & 0,841 & 0,837 & 0,643 & 0,919 & 0,903 \\
IBk & 0,697 & 0,723 & 0,739 & 0,394 & 0,687 & 0,701 \\
\midrule 
\multicolumn{7}{l}{\texttt{ClassB}} \\
MultilayerPerceptron & 0,749 & 0,797 & 0,724 & 0,496 & 0,798 & 0,796 \\
JRip & 0,756 & 0,794 & 0,75 & 0,508 & 0,768 & 0,777 \\
NaiveBayes & 0,685 & 0,69 & 0,821 & 0,387 & 0,778 & 0,761 \\
RandomForest & 0,741 & 0,769 & 0,762 & 0,482 & 0,797 & 0,793 \\
IBk & 0,732 & 0,75 & 0,785 & 0,467 & 0,754 & 0,764 \\
\midrule 
\multicolumn{7}{l}{\texttt{\texttt{\% tweets by unofficial clients}}} \\
MultilayerPerceptron & 0,529 & 0,574 & 0,632 & 0,059 & 0,575 & 0,542 \\
JRip & 0,548 & 0,58 & 0,859 & 0,123 & 0,575 & 0,545 \\
NaiveBayes & 0,538 & 0,572 & 0,925 & 0,121 & 0,578 & 0,55 \\
RandomForest & 0,545 & 0,577 & 0,872 & 0,119 & 0,577 & 0,549 \\
IBk & 0,545 & 0,577 & 0,872 & 0,119 & 0,576 & 0,548 \\

	\bottomrule
	\end{tabular}
	\caption{\small stock: 10-folds cross validation  (imbalanced, \#post > 10).}
	\label{tab:stock10}
\end{table*}

\begin{table*}[t!]
	\scriptsize
	\centering
	\begin{tabular}{lcccccc}
		\toprule
		& \multicolumn{5}{c}{\textbf{rtbust}} \\
		\cmidrule{2-7}
		Name & Bal.Accuracy & Precision & Recall & MCC & PR-AUC & ROC-AUC \\
		\midrule
ZeroR & 0,493 & 0,493 & 0,493 & -0,014 & 0,496 & 0,493 \\
\midrule 
\multicolumn{7}{l}{\texttt{CAP\_UNI}} \\
MultilayerPerceptron & 0,591 & 0,625 & 0,454 & 0,19 & 0,598 & 0,6 \\
JRip & 0,612 & 0,611 & 0,616 & 0,224 & 0,571 & 0,604 \\
NaiveBayes & 0,539 & 0,647 & 0,169 & 0,114 & 0,578 & 0,582 \\
RandomForest & 0,508 & 0,508 & 0,448 & 0,015 & 0,54 & 0,531 \\
IBk & 0,517 & 0,516 & 0,531 & 0,034 & 0,557 & 0,531 \\
\midrule 
\multicolumn{7}{l}{\texttt{ClassA}} \\
MultilayerPerceptron & 0,728 & 0,762 & 0,661 & 0,459 & 0,756 & 0,769 \\
JRip & 0,736 & 0,767 & 0,677 & 0,474 & 0,738 & 0,74 \\
NaiveBayes & 0,561 & 0,533 & 0,95 & 0,192 & 0,72 & 0,749 \\
RandomForest & 0,753 & 0,779 & 0,705 & 0,508 & 0,86 & 0,839 \\
IBk & 0,69 & 0,688 & 0,693 & 0,379 & 0,627 & 0,679 \\
\midrule 
\multicolumn{7}{l}{\texttt{ClassB}} \\
MultilayerPerceptron & 0,752 & 0,767 & 0,721 & 0,504 & 0,784 & 0,795 \\
JRip & 0,731 & 0,762 & 0,67 & 0,465 & 0,73 & 0,758 \\
NaiveBayes & 0,717 & 0,688 & 0,791 & 0,438 & 0,756 & 0,783 \\
RandomForest & 0,714 & 0,718 & 0,702 & 0,427 & 0,751 & 0,779 \\
IBk & 0,679 & 0,666 & 0,715 & 0,358 & 0,682 & 0,718 \\
\midrule 
\multicolumn{7}{l}{\texttt{\texttt{\% tweets by unofficial clients}}} \\
MultilayerPerceptron & 0,512 & 0,511 & 0,556 & 0,025 & 0,511 & 0,508 \\
JRip & 0,53 & 0,518 & 0,835 & 0,076 & 0,494 & 0,5 \\
NaiveBayes & 0,511 & 0,506 & 0,854 & 0,03 & 0,498 & 0,5 \\
RandomForest & 0,508 & 0,504 & 0,842 & 0,021 & 0,475 & 0,477 \\
IBk & 0,502 & 0,5 & 0,845 & 0,004 & 0,476 & 0,476 \\
	\bottomrule
	\end{tabular}
	\caption{\small rtbust: 10-folds cross validation  (imbalanced, \#post > 10).}
	\label{tab:rtbust10}
\end{table*}

\begin{table*}[t!]
	\scriptsize
	\centering
	\begin{tabular}{lcccccc}
		\toprule
		& \multicolumn{5}{c}{\textbf{botwiki-celebrity}} \\
		\cmidrule{2-7}
		Name & Bal.Accuracy & Precision & Recall & MCC & PR-AUC & ROC-AUC \\
		\midrule
		ZeroR & 0,5 & 0 & 0 & 0 & 0,112 & 0,499 \\
\midrule 
\multicolumn{7}{l}{\texttt{CAP\_UNI}} \\
MultilayerPerceptron & 0,856 & 0,725 & 0,748 & 0,703 & 0,698 & 0,932 \\
JRip & 0,846 & 0,744 & 0,722 & 0,7 & 0,598 & 0,85 \\
NaiveBayes & 0,7 & 0,818 & 0,41 & 0,546 & 0,716 & 0,91 \\
RandomForest & 0,836 & 0,754 & 0,701 & 0,694 & 0,724 & 0,95 \\
IBk & 0,839 & 0,752 & 0,707 & 0,696 & 0,72 & 0,95 \\
\midrule 
\multicolumn{7}{l}{\texttt{ClassA}} \\
MultilayerPerceptron & 0,956 & 0,92 & 0,921 & 0,91 & 0,972 & 0,995 \\
JRip & 0,985 & 0,977 & 0,971 & 0,971 & 0,968 & 0,984 \\
NaiveBayes & 0,979 & 0,822 & 0,985 & 0,886 & 0,976 & 0,994 \\
RandomForest & 0,988 & 0,991 & 0,978 & 0,982 & 0,998 & 1 \\
IBk & 0,951 & 0,906 & 0,913 & 0,898 & 0,829 & 0,947 \\
\midrule 
\multicolumn{7}{l}{\texttt{ClassB}} \\
MultilayerPerceptron & 0,925 & 0,89 & 0,863 & 0,861 & 0,915 & 0,958 \\
JRip & 0,95 & 0,896 & 0,913 & 0,892 & 0,879 & 0,958 \\
NaiveBayes & 0,911 & 0,519 & 0,932 & 0,647 & 0,649 & 0,944 \\
RandomForest & 0,941 & 0,9 & 0,893 & 0,884 & 0,938 & 0,992 \\
IBk & 0,922 & 0,843 & 0,864 & 0,835 & 0,689 & 0,919 \\
\midrule 
\multicolumn{7}{l}{\texttt{\texttt{\% tweets by unofficial clients}}} \\
MultilayerPerceptron & 0,954 & 0,7 & 0,959 & 0,794 & 0,719 & 0,969 \\
JRip & 0,951 & 0,714 & 0,95 & 0,799 & 0,66 & 0,942 \\
NaiveBayes & 0,946 & 0,549 & 0,994 & 0,699 & 0,69 & 0,968 \\
RandomForest & 0,951 & 0,714 & 0,95 & 0,799 & 0,677 & 0,963 \\
IBk & 0,951 & 0,714 & 0,95 & 0,799 & 0,677 & 0,964 \\
	\bottomrule
	\end{tabular}
	\caption{\small botwiki-celebrity: 10-folds cross validation  (imbalanced, \#post > 100).}
	\label{tab:botwiki-celebrity100}
\end{table*}

\begin{table*}[t!]
	\scriptsize
	\centering
	\begin{tabular}{lcccccc}
		\toprule
		& \multicolumn{5}{c}{\textbf{botwiki-verified}} \\
		\cmidrule{2-7}
		Name & Bal.Accuracy & Precision & Recall & MCC & PR-AUC & ROC-AUC \\
		\midrule
		ZeroR & 0,5 & 0 & 0 & 0 & 0,249 & 0,498 \\
\midrule 
\multicolumn{7}{l}{\texttt{CAP\_UNI}} \\
MultilayerPerceptron & 0,843 & 0,86 & 0,724 & 0,727 & 0,855 & 0,915 \\
JRip & 0,844 & 0,867 & 0,724 & 0,732 & 0,766 & 0,848 \\
NaiveBayes & 0,72 & 0,977 & 0,444 & 0,601 & 0,844 & 0,89 \\
RandomForest & 0,842 & 0,879 & 0,716 & 0,734 & 0,865 & 0,916 \\
IBk & 0,844 & 0,871 & 0,722 & 0,734 & 0,864 & 0,916 \\
\midrule 
\multicolumn{7}{l}{\texttt{ClassA}} \\
MultilayerPerceptron & 0,954 & 0,918 & 0,936 & 0,902 & 0,946 & 0,986 \\
JRip & 0,979 & 0,97 & 0,968 & 0,959 & 0,968 & 0,981 \\
NaiveBayes & 0,96 & 0,901 & 0,955 & 0,902 & 0,962 & 0,982 \\
RandomForest & 0,981 & 0,99 & 0,965 & 0,97 & 0,997 & 0,999 \\
IBk & 0,95 & 0,916 & 0,929 & 0,896 & 0,864 & 0,948 \\
\midrule 
\multicolumn{7}{l}{\texttt{ClassB}} \\
MultilayerPerceptron & 0,965 & 0,963 & 0,941 & 0,936 & 0,977 & 0,985 \\
JRip & 0,975 & 0,959 & 0,962 & 0,948 & 0,955 & 0,978 \\
NaiveBayes & 0,933 & 0,783 & 0,953 & 0,814 & 0,854 & 0,962 \\
RandomForest & 0,972 & 0,962 & 0,956 & 0,945 & 0,98 & 0,996 \\
IBk & 0,957 & 0,938 & 0,935 & 0,915 & 0,876 & 0,951 \\
\midrule 
\multicolumn{7}{l}{\texttt{\texttt{\% tweets by unofficial clients}}} \\
MultilayerPerceptron & 0,949 & 0,81 & 0,975 & 0,848 & 0,821 & 0,958 \\
JRip & 0,949 & 0,815 & 0,97 & 0,849 & 0,797 & 0,942 \\
NaiveBayes & 0,926 & 0,7 & 0,994 & 0,771 & 0,801 & 0,956 \\
RandomForest & 0,942 & 0,824 & 0,952 & 0,845 & 0,79 & 0,951 \\
IBk & 0,942 & 0,819 & 0,955 & 0,843 & 0,79 & 0,951 \\
	\bottomrule
	\end{tabular}
	\caption{\small botwiki-verified: 10-folds cross validation  (imbalanced, \#post > 100).}
	\label{tab:botwiki-verified100}
\end{table*}

\begin{table*}[t!]
	\scriptsize
	\centering
	\begin{tabular}{lcccccc}
		\toprule
		& \multicolumn{5}{c}{\textbf{vendor-verified}} \\
		\cmidrule{2-7}
		Name & Bal.Accuracy & Precision & Recall & MCC & PR-AUC & ROC-AUC \\
		\midrule
		ZeroR & 0,5 & 0 & 0 & 0 & 0,131 & 0,497 \\
\midrule 
\multicolumn{7}{l}{\texttt{CAP\_UNI}} \\
MultilayerPerceptron & 0,818 & 0,894 & 0,648 & 0,732 & 0,786 & 0,895 \\
JRip & 0,818 & 0,859 & 0,652 & 0,716 & 0,667 & 0,815 \\
NaiveBayes & 0,776 & 0,944 & 0,558 & 0,697 & 0,785 & 0,9 \\
RandomForest & 0,807 & 0,899 & 0,625 & 0,72 & 0,787 & 0,913 \\
IBk & 0,813 & 0,888 & 0,638 & 0,723 & 0,757 & 0,914 \\
\midrule 
\multicolumn{7}{l}{\texttt{ClassA}} \\
MultilayerPerceptron & 0,795 & 0,858 & 0,605 & 0,687 & 0,788 & 0,908 \\
JRip & 0,875 & 0,814 & 0,776 & 0,764 & 0,727 & 0,873 \\
NaiveBayes & 0,744 & 0,881 & 0,497 & 0,628 & 0,758 & 0,929 \\
RandomForest & 0,892 & 0,905 & 0,796 & 0,828 & 0,904 & 0,966 \\
IBk & 0,795 & 0,714 & 0,628 & 0,623 & 0,505 & 0,798 \\
\midrule 
\multicolumn{7}{l}{\texttt{ClassB}} \\
MultilayerPerceptron & 0,664 & 0,731 & 0,346 & 0,457 & 0,508 & 0,737 \\
JRip & 0,666 & 0,64 & 0,363 & 0,427 & 0,391 & 0,674 \\
NaiveBayes & 0,672 & 0,507 & 0,403 & 0,379 & 0,378 & 0,769 \\
RandomForest & 0,668 & 0,686 & 0,36 & 0,446 & 0,533 & 0,791 \\
IBk & 0,644 & 0,406 & 0,37 & 0,3 & 0,25 & 0,649 \\
\midrule 
\multicolumn{7}{l}{\texttt{\texttt{\% tweets by unofficial clients}}} \\
MultilayerPerceptron & 0,5 & 0 & 0 & 0 & 0,201 & 0,633 \\
JRip & 0,5 & 0 & 0 & 0 & 0,131 & 0,497 \\
NaiveBayes & 0,5 & 0 & 0 & 0 & 0,188 & 0,591 \\
RandomForest & 0,5 & 0 & 0 & 0 & 0,182 & 0,632 \\
IBk & 0,499 & 0 & 0 & -0,016 & 0,181 & 0,632 \\
	\bottomrule
	\end{tabular}
	\caption{\small vendor-verified: 10-folds cross validation  (imbalanced, \#post > 100).}
	\label{tab:vendor-verified100}
\end{table*}

\begin{table*}[t!]
	\scriptsize
	\centering
	\begin{tabular}{lcccccc}
		\toprule
		& \multicolumn{5}{c}{\textbf{stock}} \\
		\cmidrule{2-7}
		Name & Bal.Accuracy & Precision & Recall & MCC & PR-AUC & ROC-AUC \\
		\midrule
		ZeroR & 0,5 & 0,568 & 1 & 0 & 0,568 & 0,5 \\
\midrule 
\multicolumn{7}{l}{\texttt{CAP\_UNI}} \\
MultilayerPerceptron & 0,744 & 0,742 & 0,901 & 0,523 & 0,736 & 0,758 \\
JRip & 0,744 & 0,743 & 0,893 & 0,518 & 0,731 & 0,747 \\
NaiveBayes & 0,733 & 0,756 & 0,811 & 0,473 & 0,708 & 0,742 \\
RandomForest & 0,744 & 0,744 & 0,893 & 0,519 & 0,776 & 0,793 \\
IBk & 0,744 & 0,743 & 0,894 & 0,519 & 0,776 & 0,793 \\
\midrule 
\multicolumn{7}{l}{\texttt{ClassA}} \\
MultilayerPerceptron & 0,711 & 0,736 & 0,799 & 0,43 & 0,795 & 0,777 \\
JRip & 0,813 & 0,839 & 0,837 & 0,625 & 0,823 & 0,838 \\
NaiveBayes & 0,541 & 0,589 & 0,986 & 0,185 & 0,783 & 0,751 \\
RandomForest & 0,821 & 0,843 & 0,85 & 0,643 & 0,923 & 0,904 \\
IBk & 0,707 & 0,744 & 0,757 & 0,415 & 0,714 & 0,712 \\
\midrule 
\multicolumn{7}{l}{\texttt{ClassB}} \\
MultilayerPerceptron & 0,826 & 0,845 & 0,858 & 0,652 & 0,877 & 0,871 \\
JRip & 0,83 & 0,847 & 0,867 & 0,663 & 0,827 & 0,838 \\
NaiveBayes & 0,772 & 0,778 & 0,871 & 0,56 & 0,824 & 0,827 \\
RandomForest & 0,806 & 0,832 & 0,835 & 0,613 & 0,884 & 0,874 \\
IBk & 0,77 & 0,791 & 0,828 & 0,544 & 0,803 & 0,791 \\
\midrule 
\multicolumn{7}{l}{\texttt{\texttt{\% tweets by unofficial clients}}} \\
MultilayerPerceptron & 0,581 & 0,616 & 0,89 & 0,207 & 0,618 & 0,589 \\
JRip & 0,591 & 0,628 & 0,824 & 0,206 & 0,614 & 0,583 \\
NaiveBayes & 0,55 & 0,595 & 0,954 & 0,172 & 0,615 & 0,586 \\
RandomForest & 0,581 & 0,618 & 0,868 & 0,2 & 0,616 & 0,59 \\
IBk & 0,579 & 0,616 & 0,872 & 0,195 & 0,615 & 0,589 \\

	\bottomrule
	\end{tabular}
	\caption{\small stock: 10-folds cross validation  (imbalanced, \#post > 100).}
	\label{tab:stock100}
\end{table*}

\begin{table*}[t!]
	\scriptsize
	\centering
	\begin{tabular}{lcccccc}
		\toprule
		& \multicolumn{5}{c}{\textbf{rtbust}} \\
		\cmidrule{2-7}
		Name & Bal.Accuracy & Precision & Recall & MCC & PR-AUC & ROC-AUC \\
		\midrule
		ZeroR & 0,493 & 0,493 & 0,493 & -0,015 & 0,497 & 0,493 \\
\midrule 
\multicolumn{7}{l}{\texttt{CAP\_UNI}} \\
MultilayerPerceptron & 0,593 & 0,65 & 0,4 & 0,2 & 0,599 & 0,602 \\
JRip & 0,62 & 0,617 & 0,629 & 0,239 & 0,572 & 0,605 \\
NaiveBayes & 0,537 & 0,642 & 0,166 & 0,11 & 0,574 & 0,565 \\
RandomForest & 0,535 & 0,54 & 0,483 & 0,071 & 0,555 & 0,56 \\
IBk & 0,543 & 0,541 & 0,575 & 0,086 & 0,563 & 0,552 \\
\midrule 
\multicolumn{7}{l}{\texttt{ClassA}} \\
MultilayerPerceptron & 0,707 & 0,741 & 0,635 & 0,417 & 0,758 & 0,773 \\
JRip & 0,732 & 0,767 & 0,667 & 0,468 & 0,752 & 0,752 \\
NaiveBayes & 0,562 & 0,536 & 0,94 & 0,189 & 0,704 & 0,72 \\
RandomForest & 0,758 & 0,782 & 0,715 & 0,517 & 0,86 & 0,836 \\
IBk & 0,691 & 0,687 & 0,702 & 0,382 & 0,631 & 0,691 \\
\midrule 
\multicolumn{7}{l}{\texttt{ClassB}} \\
MultilayerPerceptron & 0,793 & 0,824 & 0,743 & 0,587 & 0,83 & 0,848 \\
JRip & 0,793 & 0,841 & 0,721 & 0,591 & 0,813 & 0,81 \\
NaiveBayes & 0,742 & 0,712 & 0,813 & 0,488 & 0,81 & 0,822 \\
RandomForest & 0,796 & 0,828 & 0,747 & 0,594 & 0,873 & 0,845 \\
IBk & 0,785 & 0,796 & 0,766 & 0,569 & 0,73 & 0,787 \\
\midrule 
\multicolumn{7}{l}{\texttt{\texttt{\% tweets by unofficial clients}}} \\
MultilayerPerceptron & 0,532 & 0,539 & 0,445 & 0,065 & 0,529 & 0,543 \\
JRip & 0,575 & 0,553 & 0,791 & 0,166 & 0,514 & 0,537 \\
NaiveBayes & 0,532 & 0,519 & 0,905 & 0,096 & 0,509 & 0,526 \\
RandomForest & 0,553 & 0,534 & 0,839 & 0,128 & 0,491 & 0,514 \\
IBk & 0,543 & 0,527 & 0,845 & 0,108 & 0,49 & 0,51 \\

	\bottomrule
	\end{tabular}
	\caption{\small rtbust: 10-folds cross validation  (imbalanced, \#post > 100).}
	\label{tab:rtbust100}
\end{table*}

---

\begin{table*}[t!]
	\scriptsize
	\centering
	\begin{tabular}{lcccccc}
		\toprule
		& \multicolumn{5}{c}{\textbf{botwiki-celebrity}} \\
		\cmidrule{2-7}
		Name & Bal.Accuracy & Precision & Recall & MCC & PR-AUC & ROC-AUC \\
		\midrule
ZeroR & 0,5 & 0 & 0 & 0 & 0,117 & 0,5 \\
\midrule 
\multicolumn{7}{l}{\texttt{CAP\_UNI}} \\
MultilayerPerceptron & 0,853 & 0,743 & 0,739 & 0,707 & 0,72 & 0,934 \\
JRip & 0,835 & 0,778 & 0,695 & 0,703 & 0,592 & 0,836 \\
NaiveBayes & 0,708 & 0,825 & 0,427 & 0,559 & 0,73 & 0,913 \\
RandomForest & 0,841 & 0,77 & 0,709 & 0,706 & 0,741 & 0,95 \\
IBk & 0,842 & 0,769 & 0,712 & 0,707 & 0,732 & 0,948 \\
\midrule 
\multicolumn{7}{l}{\texttt{ClassA}} \\
MultilayerPerceptron & 0,951 & 0,911 & 0,914 & 0,901 & 0,97 & 0,994 \\
JRip & 0,987 & 0,98 & 0,976 & 0,975 & 0,973 & 0,988 \\
NaiveBayes & 0,978 & 0,827 & 0,984 & 0,888 & 0,972 & 0,994 \\
RandomForest & 0,989 & 0,988 & 0,979 & 0,981 & 0,998 & 1 \\
IBk & 0,949 & 0,915 & 0,91 & 0,901 & 0,842 & 0,947 \\
\midrule 
\multicolumn{7}{l}{\texttt{ClassB}} \\
MultilayerPerceptron & 0,926 & 0,908 & 0,863 & 0,871 & 0,914 & 0,961 \\
JRip & 0,952 & 0,898 & 0,917 & 0,895 & 0,896 & 0,958 \\
NaiveBayes & 0,915 & 0,547 & 0,933 & 0,668 & 0,68 & 0,949 \\
RandomForest & 0,942 & 0,917 & 0,894 & 0,893 & 0,967 & 0,994 \\
IBk & 0,933 & 0,874 & 0,883 & 0,862 & 0,883 & 0,938 \\
\midrule 
\multicolumn{7}{l}{\texttt{\texttt{\% tweets by unofficial clients}}} \\
MultilayerPerceptron & 0,957 & 0,741 & 0,957 & 0,819 & 0,779 & 0,973 \\
JRip & 0,946 & 0,772 & 0,928 & 0,825 & 0,722 & 0,942 \\
NaiveBayes & 0,947 & 0,572 & 0,993 & 0,715 & 0,733 & 0,971 \\
RandomForest & 0,945 & 0,78 & 0,925 & 0,828 & 0,734 & 0,968 \\
IBk & 0,945 & 0,78 & 0,925 & 0,828 & 0,734 & 0,97 \\

	\bottomrule
	\end{tabular}
	\caption{\small botwiki-celebrity: 10-folds cross validation  (imbalanced, \#post > 200).}
	\label{tab:botwiki-celebrity200}
\end{table*}

\begin{table*}[t!]
	\scriptsize
	\centering
	\begin{tabular}{lcccccc}
		\toprule
		& \multicolumn{5}{c}{\textbf{botwiki-verified}} \\
		\cmidrule{2-7}
		Name & Bal.Accuracy & Precision & Recall & MCC & PR-AUC & ROC-AUC \\
		\midrule
ZeroR & 0,5 & 0 & 0 & 0 & 0,249 & 0,499 \\
\midrule 
\multicolumn{7}{l}{\texttt{CAP\_UNI}} \\
MultilayerPerceptron & 0,836 & 0,874 & 0,705 & 0,724 & 0,847 & 0,909 \\
JRip & 0,833 & 0,864 & 0,702 & 0,716 & 0,745 & 0,831 \\
NaiveBayes & 0,717 & 0,966 & 0,438 & 0,592 & 0,841 & 0,89 \\
RandomForest & 0,844 & 0,868 & 0,725 & 0,733 & 0,865 & 0,918 \\
IBk & 0,844 & 0,86 & 0,728 & 0,73 & 0,863 & 0,918 \\
\midrule 
\multicolumn{7}{l}{\texttt{ClassA}} \\
MultilayerPerceptron & 0,949 & 0,929 & 0,922 & 0,901 & 0,935 & 0,984 \\
JRip & 0,977 & 0,968 & 0,965 & 0,955 & 0,963 & 0,979 \\
NaiveBayes & 0,964 & 0,909 & 0,959 & 0,91 & 0,967 & 0,984 \\
RandomForest & 0,984 & 0,99 & 0,971 & 0,974 & 0,998 & 0,999 \\
IBk & 0,952 & 0,912 & 0,934 & 0,897 & 0,873 & 0,953 \\
\midrule 
\multicolumn{7}{l}{\texttt{ClassB}} \\
MultilayerPerceptron & 0,965 & 0,957 & 0,943 & 0,934 & 0,976 & 0,982 \\
JRip & 0,98 & 0,954 & 0,976 & 0,953 & 0,953 & 0,987 \\
NaiveBayes & 0,936 & 0,795 & 0,954 & 0,824 & 0,86 & 0,964 \\
RandomForest & 0,98 & 0,968 & 0,97 & 0,958 & 0,991 & 0,997 \\
IBk & 0,965 & 0,947 & 0,948 & 0,93 & 0,952 & 0,97 \\
\midrule 
\multicolumn{7}{l}{\texttt{\texttt{\% tweets by unofficial clients}}} \\
MultilayerPerceptron & 0,951 & 0,846 & 0,96 & 0,866 & 0,856 & 0,966 \\
JRip & 0,954 & 0,855 & 0,962 & 0,874 & 0,83 & 0,949 \\
NaiveBayes & 0,931 & 0,715 & 0,993 & 0,783 & 0,841 & 0,964 \\
RandomForest & 0,954 & 0,86 & 0,96 & 0,877 & 0,843 & 0,963 \\
IBk & 0,953 & 0,855 & 0,96 & 0,873 & 0,845 & 0,964 \\

	\bottomrule
	\end{tabular}
	\caption{\small botwiki-verified: 10-folds cross validation  (imbalanced, \#post > 200).}
	\label{tab:botwiki-verified200}
\end{table*}

\begin{table*}[t!]
	\scriptsize
	\centering
	\begin{tabular}{lcccccc}
		\toprule
		& \multicolumn{5}{c}{\textbf{vendor-verified}} \\
		\cmidrule{2-7}
		Name & Bal.Accuracy & Precision & Recall & MCC & PR-AUC & ROC-AUC \\
		\midrule
ZeroR & 0,5 & 0 & 0 & 0 & 0,11 & 0,496 \\
\midrule 
\multicolumn{7}{l}{\texttt{CAP\_UNI}} \\
MultilayerPerceptron & 0,781 & 0,864 & 0,573 & 0,675 & 0,735 & 0,88 \\
JRip & 0,786 & 0,813 & 0,589 & 0,661 & 0,6 & 0,793 \\
NaiveBayes & 0,727 & 0,941 & 0,457 & 0,631 & 0,719 & 0,867 \\
RandomForest & 0,774 & 0,845 & 0,56 & 0,659 & 0,729 & 0,888 \\
IBk & 0,773 & 0,835 & 0,56 & 0,654 & 0,722 & 0,89 \\
\midrule 
\multicolumn{7}{l}{\texttt{ClassA}} \\
MultilayerPerceptron & 0,769 & 0,818 & 0,552 & 0,64 & 0,703 & 0,846 \\
JRip & 0,849 & 0,792 & 0,721 & 0,727 & 0,687 & 0,847 \\
NaiveBayes & 0,781 & 0,864 & 0,573 & 0,675 & 0,74 & 0,912 \\
RandomForest & 0,872 & 0,868 & 0,758 & 0,79 & 0,87 & 0,963 \\
IBk & 0,754 & 0,672 & 0,54 & 0,559 & 0,433 & 0,77 \\
\midrule 
\multicolumn{7}{l}{\texttt{ClassB}} \\
MultilayerPerceptron & 0,602 & 0,545 & 0,227 & 0,304 & 0,367 & 0,718 \\
JRip & 0,606 & 0,559 & 0,235 & 0,316 & 0,263 & 0,596 \\
NaiveBayes & 0,628 & 0,391 & 0,317 & 0,281 & 0,309 & 0,75 \\
RandomForest & 0,622 & 0,576 & 0,268 & 0,345 & 0,412 & 0,782 \\
IBk & 0,594 & 0,306 & 0,26 & 0,201 & 0,174 & 0,604 \\
\midrule 
\multicolumn{7}{l}{\texttt{\texttt{\% tweets by unofficial clients}}} \\
MultilayerPerceptron & 0,5 & 0 & 0 & 0 & 0,152 & 0,574 \\
JRip & 0,5 & 0 & 0 & 0 & 0,11 & 0,496 \\
NaiveBayes & 0,5 & 0 & 0 & 0 & 0,135 & 0,58 \\
RandomForest & 0,498 & 0 & 0 & -0,022 & 0,124 & 0,562 \\
IBk & 0,493 & 0 & 0 & -0,04 & 0,126 & 0,563 \\

	\bottomrule
	\end{tabular}
	\caption{\small vendor-verified: 10-folds cross validation  (imbalanced, \#post > 200).}
	\label{tab:vendor-verified200}
\end{table*}

\begin{table*}[t!]
	\scriptsize
	\centering
	\begin{tabular}{lcccccc}
		\toprule
		& \multicolumn{5}{c}{\textbf{stock}} \\
		\cmidrule{2-7}
		Name & Bal.Accuracy & Precision & Recall & MCC & PR-AUC & ROC-AUC \\
		\midrule
ZeroR & 0,5 & 0,586 & 1 & 0 & 0,586 & 0,5 \\
\midrule 
\multicolumn{7}{l}{\texttt{CAP\_UNI}} \\
MultilayerPerceptron & 0,775 & 0,784 & 0,9 & 0,576 & 0,789 & 0,795 \\
JRip & 0,774 & 0,784 & 0,9 & 0,575 & 0,773 & 0,776 \\
NaiveBayes & 0,765 & 0,807 & 0,801 & 0,529 & 0,789 & 0,799 \\
RandomForest & 0,775 & 0,786 & 0,896 & 0,575 & 0,803 & 0,814 \\
IBk & 0,775 & 0,786 & 0,897 & 0,576 & 0,802 & 0,814 \\
\midrule 
\multicolumn{7}{l}{\texttt{ClassA}} \\
MultilayerPerceptron & 0,71 & 0,75 & 0,795 & 0,426 & 0,806 & 0,775 \\
JRip & 0,794 & 0,824 & 0,841 & 0,59 & 0,815 & 0,815 \\
NaiveBayes & 0,548 & 0,61 & 0,986 & 0,207 & 0,813 & 0,775 \\
RandomForest & 0,811 & 0,84 & 0,851 & 0,623 & 0,92 & 0,893 \\
IBk & 0,687 & 0,739 & 0,749 & 0,375 & 0,706 & 0,689 \\
\midrule 
\multicolumn{7}{l}{\texttt{ClassB}} \\
MultilayerPerceptron & 0,823 & 0,838 & 0,889 & 0,656 & 0,873 & 0,867 \\
JRip & 0,828 & 0,843 & 0,89 & 0,665 & 0,829 & 0,837 \\
NaiveBayes & 0,785 & 0,797 & 0,89 & 0,59 & 0,846 & 0,841 \\
RandomForest & 0,807 & 0,832 & 0,859 & 0,618 & 0,886 & 0,871 \\
IBk & 0,768 & 0,8 & 0,828 & 0,539 & 0,8 & 0,784 \\
\midrule 
\multicolumn{7}{l}{\texttt{\texttt{\% tweets by unofficial clients}}} \\
MultilayerPerceptron & 0,604 & 0,648 & 0,888 & 0,256 & 0,655 & 0,617 \\
JRip & 0,618 & 0,665 & 0,823 & 0,26 & 0,656 & 0,62 \\
NaiveBayes & 0,555 & 0,615 & 0,958 & 0,191 & 0,65 & 0,607 \\
RandomForest & 0,603 & 0,65 & 0,868 & 0,246 & 0,655 & 0,623 \\
IBk & 0,6 & 0,648 & 0,87 & 0,241 & 0,654 & 0,622 \\

	\bottomrule
	\end{tabular}
	\caption{\small stock: 10-folds cross validation  (imbalanced, \#post > 200).}
	\label{tab:stock200}
\end{table*}

\begin{table*}[t!]
	\scriptsize
	\centering
	\begin{tabular}{lcccccc}
		\toprule
		& \multicolumn{5}{c}{\textbf{rtbust}} \\
		\cmidrule{2-7}
		Name & Bal.Accuracy & Precision & Recall & MCC & PR-AUC & ROC-AUC \\
		\midrule
ZeroR & 0,5 & 0,501 & 1 & 0 & 0,497 & 0,493 \\
\midrule 
\multicolumn{7}{l}{\texttt{CAP\_UNI}} \\
MultilayerPerceptron & 0,578 & 0,611 & 0,429 & 0,163 & 0,603 & 0,602 \\
JRip & 0,617 & 0,616 & 0,626 & 0,234 & 0,579 & 0,607 \\
NaiveBayes & 0,54 & 0,648 & 0,175 & 0,116 & 0,594 & 0,587 \\
RandomForest & 0,532 & 0,533 & 0,518 & 0,063 & 0,552 & 0,551 \\
IBk & 0,541 & 0,54 & 0,569 & 0,082 & 0,569 & 0,547 \\
\midrule 
\multicolumn{7}{l}{\texttt{ClassA}} \\
MultilayerPerceptron & 0,694 & 0,726 & 0,623 & 0,391 & 0,752 & 0,753 \\
JRip & 0,724 & 0,746 & 0,68 & 0,449 & 0,699 & 0,733 \\
NaiveBayes & 0,644 & 0,6 & 0,867 & 0,321 & 0,735 & 0,755 \\
RandomForest & 0,776 & 0,803 & 0,734 & 0,554 & 0,862 & 0,84 \\
IBk & 0,69 & 0,689 & 0,696 & 0,38 & 0,63 & 0,684 \\
\midrule 
\multicolumn{7}{l}{\texttt{ClassB}} \\
MultilayerPerceptron & 0,808 & 0,844 & 0,756 & 0,619 & 0,854 & 0,843 \\
JRip & 0,796 & 0,861 & 0,705 & 0,6 & 0,836 & 0,832 \\
NaiveBayes & 0,767 & 0,736 & 0,832 & 0,538 & 0,823 & 0,836 \\
RandomForest & 0,802 & 0,826 & 0,766 & 0,605 & 0,901 & 0,874 \\
IBk & 0,792 & 0,79 & 0,797 & 0,584 & 0,746 & 0,796 \\
\midrule 
\multicolumn{7}{l}{\texttt{\texttt{\% tweets by unofficial clients}}} \\
MultilayerPerceptron & 0,552 & 0,543 & 0,674 & 0,107 & 0,543 & 0,562 \\
JRip & 0,593 & 0,569 & 0,781 & 0,201 & 0,54 & 0,567 \\
NaiveBayes & 0,534 & 0,52 & 0,915 & 0,104 & 0,523 & 0,537 \\
RandomForest & 0,566 & 0,544 & 0,829 & 0,155 & 0,527 & 0,549 \\
IBk & 0,558 & 0,538 & 0,842 & 0,14 & 0,527 & 0,543 \\

	\bottomrule
	\end{tabular}
	\caption{\small rtbust: 10-folds cross validation  (imbalanced, \#post > 200).}
	\label{tab:rtbust200}
\end{table*}
